# Supplementary material for: Accelerating reactive-flow simulations using vectorized chemistry integration
Source: arXiv:2205.05681 ancillary file (2022-05-10)
Supplement: Supplementary file 1 [file supplemental.pdf]

# Supplemental material for "Accelerating reactive-flow simulations using vectorized chemistry integration"

Nicholas J. Curtis,[1] Kyle E. Niemeyer,[2] and Chih-Jen Sung[1]

[1]*Department of Mechanical Engineering, University of Connecticut, Storrs, CT 06269, USA*
[2]*School of Mechanical, Industrial, and Manufacturing Engineering, Oregon State University, Corvallis, OR 97331, USA*[*]

This document supplements the work "Accelerating reactive-flow simulations using vectorized chemistry integration" with additional comparisons of the Sandia Flame D case between `OpenFOAM` and `accelerInt` solvers, and validation of the Volvo bluff-body stabilized flame case against experimental measurements.

## S1. REACTIVE SANDIA FLAME D COMPARISON

To compare the predicted solutions of the `OpenFOAM` and `accelerInt` solvers in this setting, the solution state was sampled along several lines (pictured in Fig. 3a) cutting through the plane of the flame (Fig. 3b) both vertically and axially. The vertical sample lines are evenly spaced at intervals of 0.1 m extending downwards from the center-line to the bottom of the domain, with the first occurring at 0.1 m from the end of the jet; the axial sample line extends from the nozzle to the far right end of the domain.

Figures S.1a to S.1d compare the steady-state and time-dependent (sampled at the final state of $t = 0.01$ s) temperature and mass-fraction profiles of $CH_4$, OH, and NO across the flame for the three different solvers: `accelerInt`'s 4th-order linearly-implicit Rosenbrock method (`ROS4`), `OpenFOAM`'s `ROS4` solver, and `OpenFOAM`'s `Seulex` implementation, a linearly-implicit extrapolation Euler integration method [1]. Overall all three solvers agree well qualitatively and quantitatively for each quantity, demonstrating that `accelerInt`-coupling can accurately reproduce the solutions of the built-in `OpenFOAM` solver for temperature, as well as major and minor species.

However, certain discrepancies do exist between the predicted solutions. For example, Fig. S.1c shows that the steady-state solution computed by `OpenFOAM`'s `Seulex` solver predicts larger amounts of OH near the wall of the domain (i.e., at more than ∼0.1 m from the center-line), while the `OpenFOAM` `ROS4` solver agrees closer with `accelerInt`. For this sample, the temperature is lower than 500 K for all points more than ∼0.06 m from the centerline, hence the solution in this region is dominated by convective and mixing processes, as chemical reactions are largely inactive at such low temperatures.

These results demonstrate that it is difficult to predict how small discrepancies in the integrated thermochemical state vectors—like those computed in higher-temperature regions where chemistry is more active—might grow or interact over thousands of CFD time steps. This is true even when comparing two ODE integrators—in this case `OpenFOAM`'s `ROS4` and `Seulex` methods—that use identical tolerances and implementations of the chemical-kinetic source terms and Jacobian matrix, since each use and modify the state vectors with complex (often nonlinear) numerical methods.

Nonetheless, we will use the norms from Eqs. (23) and (24) to obtain a sense of the similarity of the solutions computed by the various solvers. However, here these norms will be labeled the mean and maximum percent differences, both because we do not have a true reference solution to compare with, but also to re-emphasize that we expect minor differences in the solutions when coupled to a full CFD solver. Additionally, since the `accelerInt` solver agrees far better with `Cantera` for constant-pressure homogeneous ignition problems (Section 3.2), we will use `accelerInt` as the "reference" solution. Further, when computing these percent differences, we excluded all points where the temperature (as predicted by `accelerInt`) is less than 500 K, since the chemistry is unimportant in these locations, and when considering all locations we observed differences (Fig. S.1c) even among the `OpenFOAM` solvers, as previously discussed.

Table S.1 shows that the mean percent difference between the `OpenFOAM` solvers and the `accelerInt` solver is roughly ∼5 %, while the maximum percent difference reaches ∼34 % in some cases. However, the maximum percent difference in temperature and pressure is significantly lower, at just ∼0.8 % and $6 \times 10^{-4}$ %, respectively. If we compare the `OpenFOAM` solvers directly—that is, if the `OpenFOAM` `ROS4` solver is used for the reference solution in calculating the percent-difference norms—the maximum and mean percent difference of the `OpenFOAM` `Seulex` solver are roughly ∼6 % and ∼0.3 %, respectively. Once again, this demonstrates that even while solving chemical kinetic ODEs with the same

[*] kyle.niemeyer@oregonstate.edu

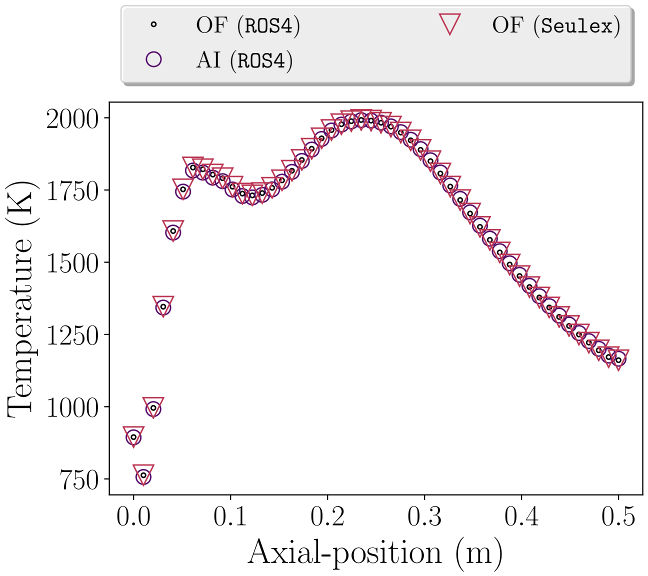


(a) The steady-state temperature solution profiles along the axial sample line extending from the nozzle to the edge of the domain.

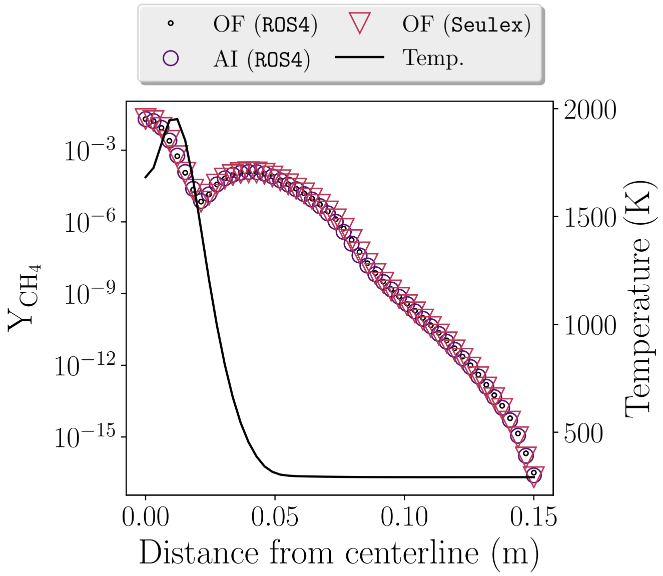


(b) The time-dependent solution profiles of the mass fraction of $CH_4$ sampled at 0.2 m away from the nozzle (i.e., the second sample line in Fig. 3c) for $t = 0.01$ s. The temperature of the flame along the same line is plotted as well to give a sense of the flame width, obtained using `AI (ROS4)`.

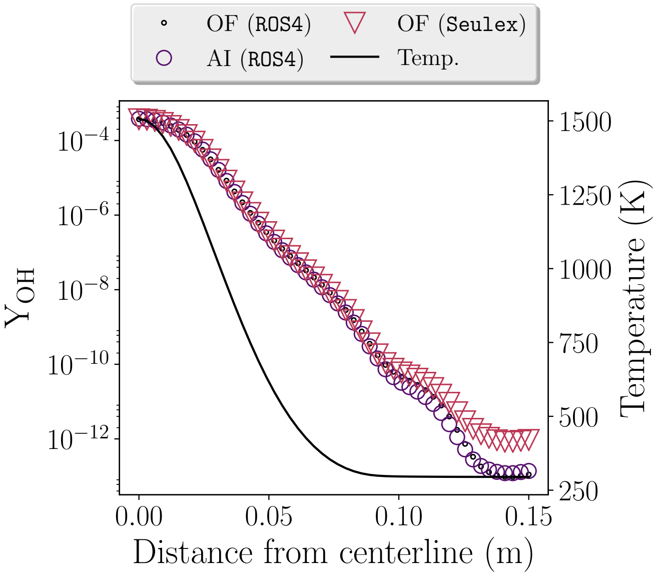


(c) The steady-state solution profiles of the mass fraction of OH sampled at 0.4 m away from the nozzle (i.e., the fourth sample line in Fig. 3c). The temperature of the flame along the same line is plotted as well to give a sense of the flame width, obtained using `AI (ROS4)`.

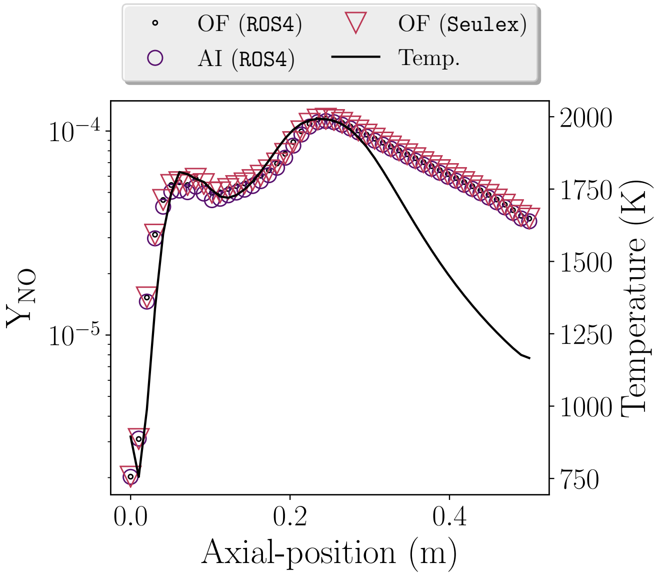


(d) The time-dependent solution profiles of the mass fraction of NO along the axial sample line extending from the nozzle to the edge of the domain for $t = 0.01$ s. The temperature of the flame along the same line is plotted as well for comparison purposes, obtained using `AI (ROS4)`.

Figure S.1: Temperature and species profile comparisons for both the steady-state and time-dependent solutions, along various sampling lines pictured in Fig. 3a. "OF" denotes an `OpenFOAM` solver, while "AI" marks the `accelerInt` version.

implementation of the chemistry evaluations and nominal tolerances, changing the integration method may lead to slightly different answers. Overall, we conclude that the three solvers agree well overall.

| | Steady-state | | Time-dependent | |
|---|---|---|---|---|
| Solver | `OpenFOAM-Seulex` | `OpenFOAM-ROS4` | `OpenFOAM-Seulex` | `OpenFOAM-ROS4` |
| $\|D\|_{\text{mean}}$ | $5.34 \times 10^{0}$ % | $5.38 \times 10^{0}$ % | $5.60 \times 10^{0}$ % | $5.63 \times 10^{0}$ % |
| $\|D\|_{\infty}$ | $2.78 \times 10^{1}$ % | $2.79 \times 10^{1}$ % | $3.43 \times 10^{1}$ % | $3.40 \times 10^{1}$ % |
| $\|D\|_{T,\infty}$ | $8.15 \times 10^{-1}$ % | $8.04 \times 10^{-1}$ % | $8.22 \times 10^{-1}$ % | $8.09 \times 10^{-1}$ % |
| $\|D\|_{p,\infty}$ | $3.86 \times 10^{-4}$ % | $3.97 \times 10^{-4}$ % | $5.63 \times 10^{-4}$ % | $6.22 \times 10^{-4}$ % |

Table S.1: Comparison of the mean and maximum percent-differences of the `OpenFOAM` solvers to `accelerInt`, using the norms defined analogously to those in Eqs. (23) and (24). The $\|D\|_{T,\infty}$ and $\|D\|_{p,\infty}$ values are the maximum percent differences in the temperature and pressure, respectively.

## S2. NON-REACTIVE EXPERIMENTAL VOLVO BLUFF-BODY STABILIZED FLAME COMPARISON

To establish the validity of the computational mesh, discretization, and numerical models used in the Volvo bluff-body stabilized flame case study, we first compare the results of the non-reactive simulation to experimental velocity and second-order turbulence statistics measurements [2–6] (as archived by Comer [7]). To do so, we initialized the simulation using a potential-flow solution and ran it for about five flow-through times, $\tau$, where

$$\tau = \frac{0.882\,\text{m}}{U_{\text{bulk}}} \sim 0.05\,\text{s}\ , \tag{S.1}$$

using a RANS turbulence model with a standard $k$–$\varepsilon$ formulation on a coarser cell grid (4 mm, ∼250,000 cells) generated similarly to that in Fig. 5b.

After the RANS simulation completed, we mapped the flowfield onto the previously discussed mesh (Fig. 5b) and ran the LES for an additional $10\,\tau$ with fixed CFD time-step size of $\Delta t = 5 \times 10^{-7}$ s, resulting in a maximum Courant number of ∼0.01 in the domain. The simulated velocity statistics used for comparison to the experimental data presented in this section were calculated using only the final $5\,\tau$ of simulated time in the LES case.

Figure S.2a compares the simulated mean axial velocity, normalized by the bulk inlet velocity, with the experimentally measured value for several axial (x-axis) locations downstream of the bluff body. We computed the simulated mean axial velocity, $\bar{u}$, using

$$\bar{u} = \frac{1}{t_2 - t_1} \int_{t1}^{t2} u\, dt\ , \tag{S.2}$$

where $t_1$ and $t_2$ are the start and end times of the velocity sampling window described previously, with $t_2 - t_1 = 5\tau$; the integration used a composite Simpson's rule algorithm in the `scipy` library [8]. The computational results do a reasonably good job of predicting the experimental velocity profiles, capturing the strength and location of the recirculation zone downstream of the bluff body with only marginal discrepancies from the experimental data, e.g., minor underpredictions of the velocity outside of the bluff-body wake. Further, the simulations well-predict the transition of a recirculation zone with sharp velocity gradients (i.e., for locations $x/D = 0.375$ to 1.53) to a smoother more-uniform velocity field downstream ($x/D = 3.75$ to 9.4).

Figure S.2b shows good agreement between the simulated and experimental mean transverse ($y$-axis) velocities $\bar{v}$, computed analogously to Eq. (S.2), for most axial locations. Near the bluff body ($x/D = 0.375$ to 0.95), the simulations capture the asymmetric peaks in the transverse velocity, and similarly well-predict the downstream ($x/D = 3.75$ to 9.4) uniform velocity profile. However, at $x/D = 1.53$ the simulated mean transverse-velocity peaks noticeably disagree with the experimental results. Another recent study by Lee and Cant [9] of the Volvo bluff-body configuration using `OpenFOAM` predicted a similar mean transverse velocity profile at $x/D = 1.53$ to that shown here; they suggested that the discrepancy resulted from mesh stretching in the downstream region or the numerical diffusion of the Smagorinsky subgrid-scale model. Considering the differences in meshing strategy and numerical discretization between the two studies, we cannot conclude on the cause of this phenomenon. We used the Smagorinsky subgrid model here, and this could indeed be the cause of the discrepancy. Further refinement of the simulated velocity profiles for better agreement with the experimental results—particularly relating to mesh stretching and subgrid model selection in `OpenFOAM`—should be investigated in future work.

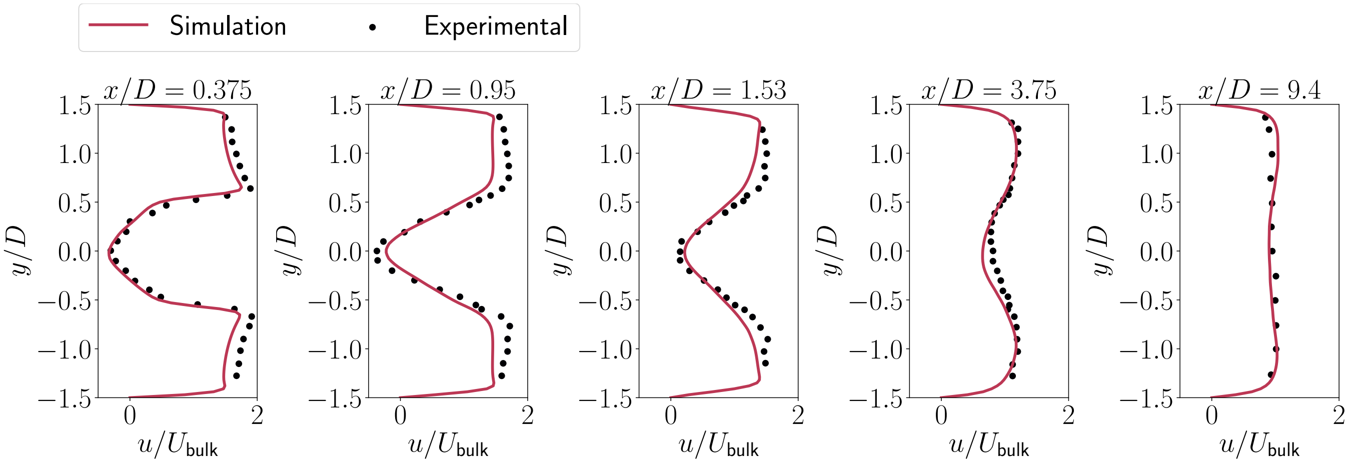


(a) The mean normalized axial velocity downstream of the bluff-body.

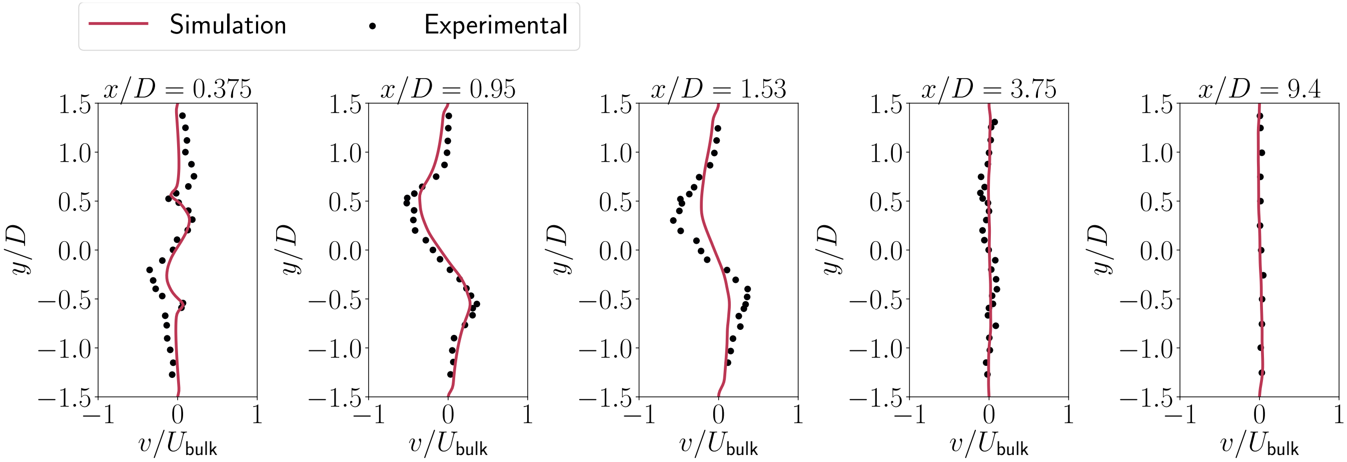


(b) The mean normalized transverse velocity downstream of the bluff-body.

Figure S.2: Comparison of the simulated mean normalized (a) axial and (b) transverse velocities to the experimental measurements at several axial locations downstream of the bluff body (here presented in multiples of the bluff-body height $D$) for the non-reactive LES case. The mean values were computed over ∼5 flow-through times (0.25 s) of the combustor at sample interval of $5 \times 10^{-4}$ s of simulated time.

To compare turbulence statistics to the experimental data, the root mean square (RMS) axial velocity fluctuation was calculated as

$$u'_{\mathrm{rms}} = \sqrt{\frac{1}{t_2 - t_1} \int_{t1}^{t2} u'(t)^2 \, \mathrm{d}t} \ , \tag{S.3}$$

and, similarly, for the transverse velocity

$$v'_{\mathrm{rms}} = \sqrt{\frac{1}{t_2 - t_1} \int_{t1}^{t2} v'(t)^2 \, \mathrm{d}t} \ . \tag{S.4}$$

The fluctuating velocities themselves were calculated as

$$u'(t) = u(t) - \bar{u} \text{ and} \tag{S.5}$$

$$v'(t) = v(t) - \bar{v} \ , \tag{S.6}$$

where $\bar{u}$ and $\bar{v}$ are computed by integral averaging as in Eq. (S.2). In addition, we computed the normalized Reynolds

stress of the transverse and axial velocities with

$$R_{xy} = \frac{\overline{u'v'}}{U_{\text{bulk}}^2} , \tag{S.7}$$

where $\overline{u'v'}$ indicates the time-averaged product of Eqs. (S.5) and (S.6).

Figure S.3 compares the normalized simulated velocity fluctuations with the experimentally measured values. The simulated axial RMS velocity fluctuations tend to slightly over-predict the fluctuation velocity outside of the bluff-body wake and underestimate the peak fluctuations near the centerline of the domain (Fig. S.3a); however, the experimental and simulated results agree well overall. Similarly, Fig. S.3b shows that the simulated transverse velocity fluctuations agree quite well with the experimentally measured values, and only slightly over- or under-predict the peak fluctuating velocities depending on the axial location. The normalized Reynolds stresses (Fig. S.3c) again show good agreement between the simulated and experimental values, with slight discrepancies at the asymmetric peak stresses.


[1] E. Hairer and G. Wanner, *Solving Ordinary Differential Equations II: Stiff and Differential-Algebraic Problems*, 2nd ed. (Springer-Verlag, Berlin, 1996).

[2] A. Sjunnesson, C. Nelsson, and E. Max, in *Fourth International Conference on Laser Anemometry – Advances and Application*, Vol. 3 (Cleveland, OH, 1991) pp. 83–90.

[3] A. Sjunnesson, S. Olovsson, and B. Sjoblom, in *International Symposium on Air Breathing Engines, 10th, Nottingham, England* (1991) pp. 385–393.

[4] A. Sjunnesson, P. Henrikson, and C. Lofstrom, in *28th Joint Propulsion Conference and Exhibit* (AIAA, 1992) AIAA Paper No. 92-3650.

[5] C. Fureby and S.-I. Moller, AIAA J. **33**, 2339 (1995).

[6] N. Zettervall, K. Nordin-Bates, E. Nilsson, and C. Fureby, Combust. Flame **179**, 1 (2017).

[7] A. Comer, Model validation for propulsion workshop - experimental data archives (2016), accessed: 01-08-19.

[8] E. Jones, T. Oliphant, P. Peterson, *et al.*, SciPy: Open source scientific tools for Python (2001–), [Online; accessed 12/02/18].

[9] C. Y. Lee and S. Cant, Combust. Theor. Model. **21**, 722 (2017).

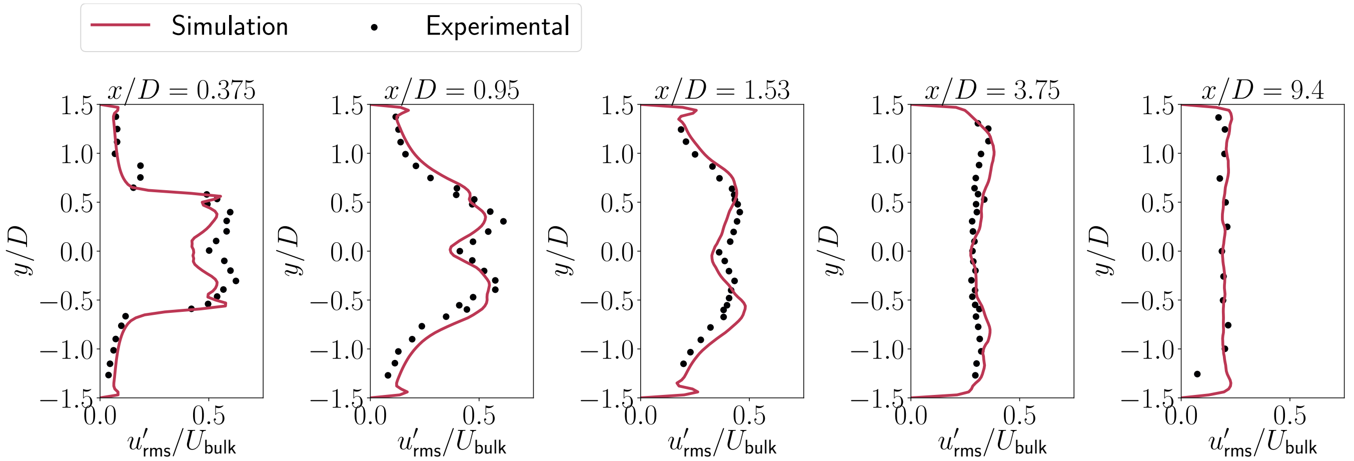


(a) The normalized RMS axial velocity fluctuations downstream of the bluff-body.

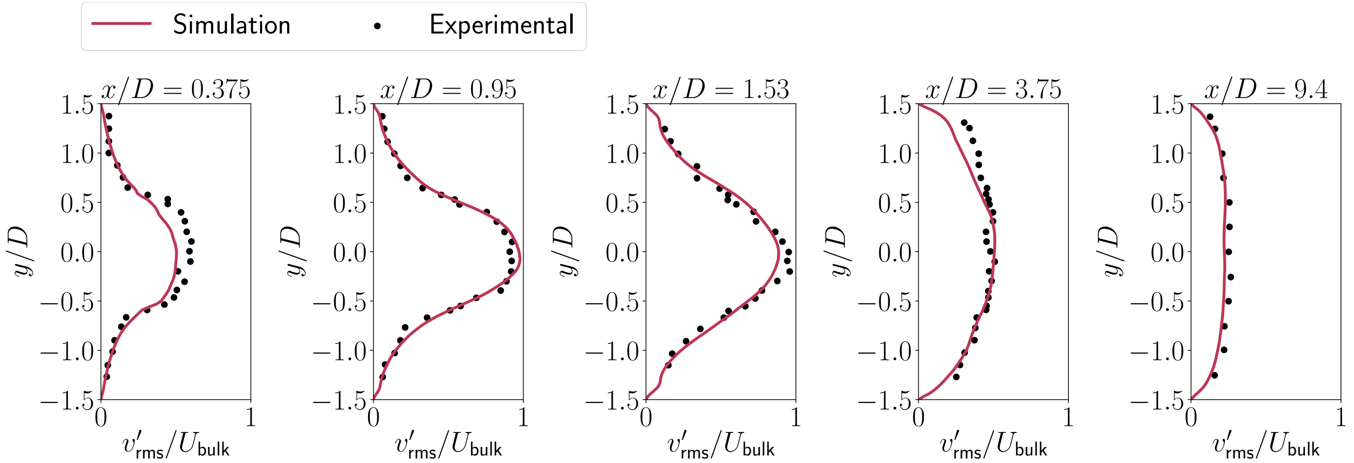


(b) The normalized RMS transverse velocity fluctuations downstream of the bluff-body.

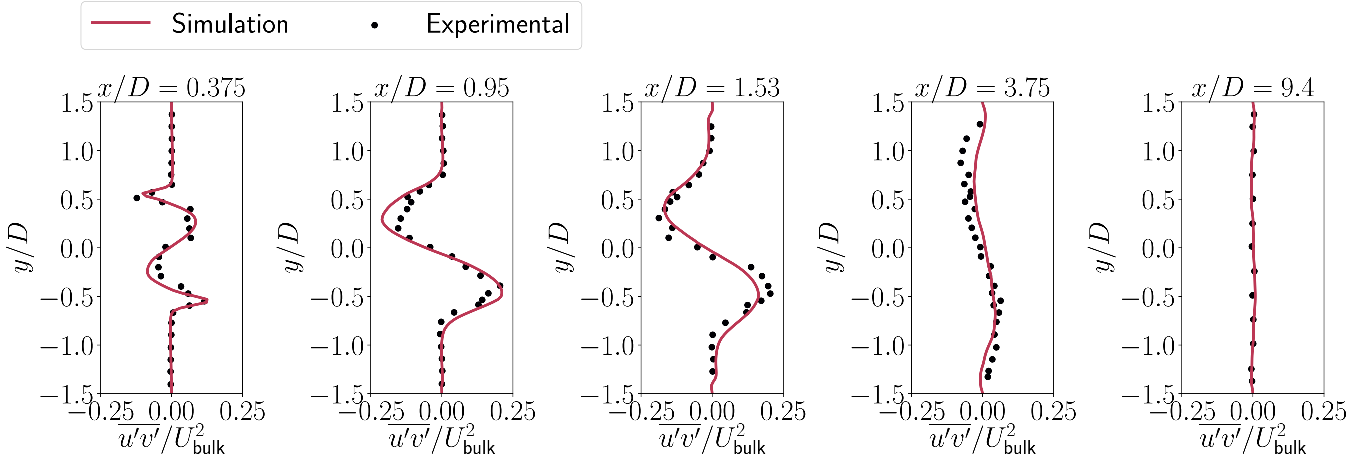


(c) The normalized time-averaged Reynolds stress downstream of the bluff-body.

Figure S.3: Comparison of the simulated RMS axial and transverse velocity fluctuations and mean Reynolds stress to the experimental measurements at several axial locations downstream of the bluff body (here presented in multiples of the bluff-body height $D$) for the non-reactive LES case. These values were computed over ∼5 flow-through times (0.25 s) of the combustor at sample interval of $5 \times 10^{-4}$ s of simulated time.
